# Supplementary material for: Toward Accurate and Temporally Consistent Video Restoration from Raw Data
Source: arXiv:2312.16247 source file (2023-12-25)
Supplement: Supplementary file 1 [file X_suppl.tex]

\clearpage
\setcounter{page}{1}
\maketitlesupplementary
\appendix

%\section{More Visual Results}
\label{sec:supp}
In this supplementary material, we first present more visual results from the REDS4 dataset (see \cref{fig:supp_Reds4_2,fig:supp_Reds4_3}) and the 4KPix50 dataset (see \cref{fig:supp_4kpix_1,fig:supp_4kpix_2}). We can see that our proposed method yields cleaner and more detailed results for both 720p and 4K video content.

% In addition, to better evaluate the temporal consistency of our method, we provide four video clips in this supplementary material, including the scenes  shown in \cref{fig:tc_compare,fig:supp_4kpix_1}. One can see that our method excels at restoring texture and details consistently throughout the sequence.

%\vspace{-100cm}
%%% -------- REDS4 results on high noise level: 02 --------

\begin{figure*}
\centering
% Patch 2
\begin{minipage}[b]{0.95\textwidth}
\centering
    \begin{minipage}[b]{0.24\textwidth}
    \centering
    \includegraphics[width=1\textwidth]{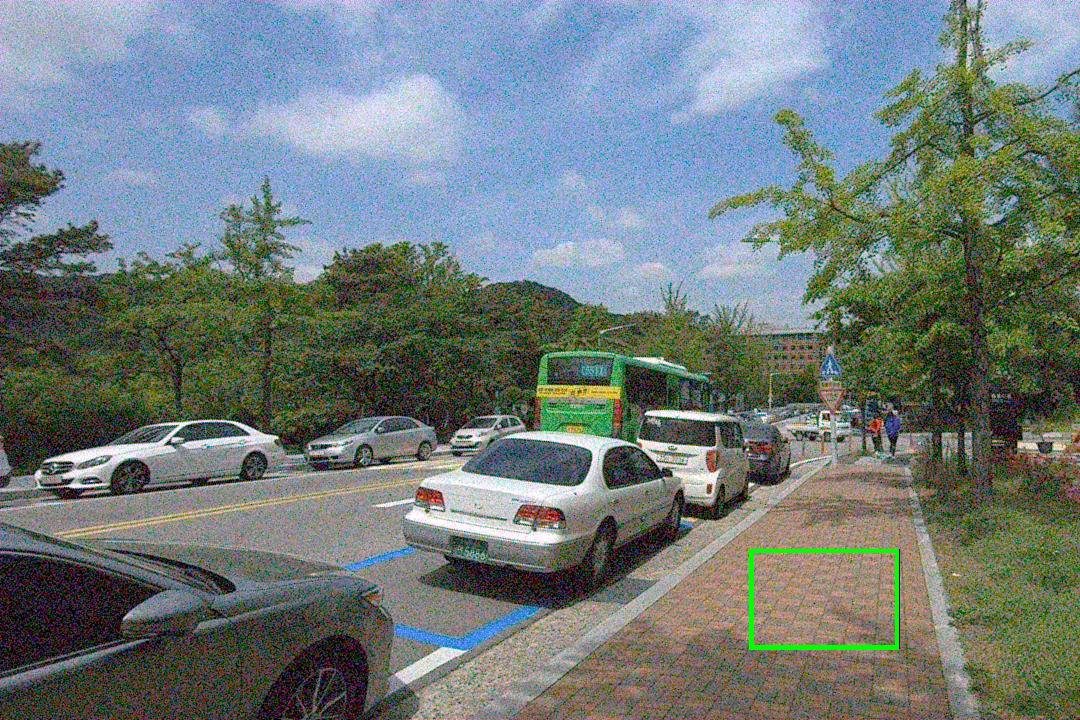}
    {\small (a) Noise image}
    \end{minipage} %\hspace{0.1cm}
    \begin{minipage}[b]{0.24\textwidth}
    \centering
    \includegraphics[width=1\textwidth]{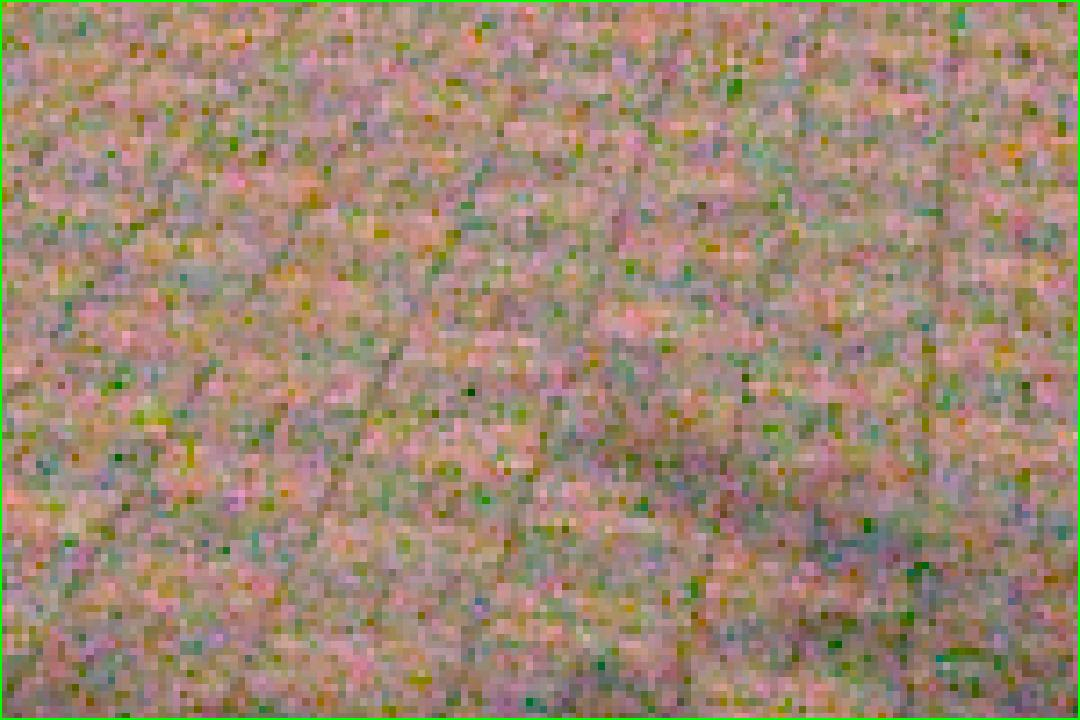}
    {\small (b) Noise patch}
    \end{minipage} %\hspace{0.1cm}
    \begin{minipage}[b]{0.24\textwidth}
    \centering
    \includegraphics[width=1\textwidth]{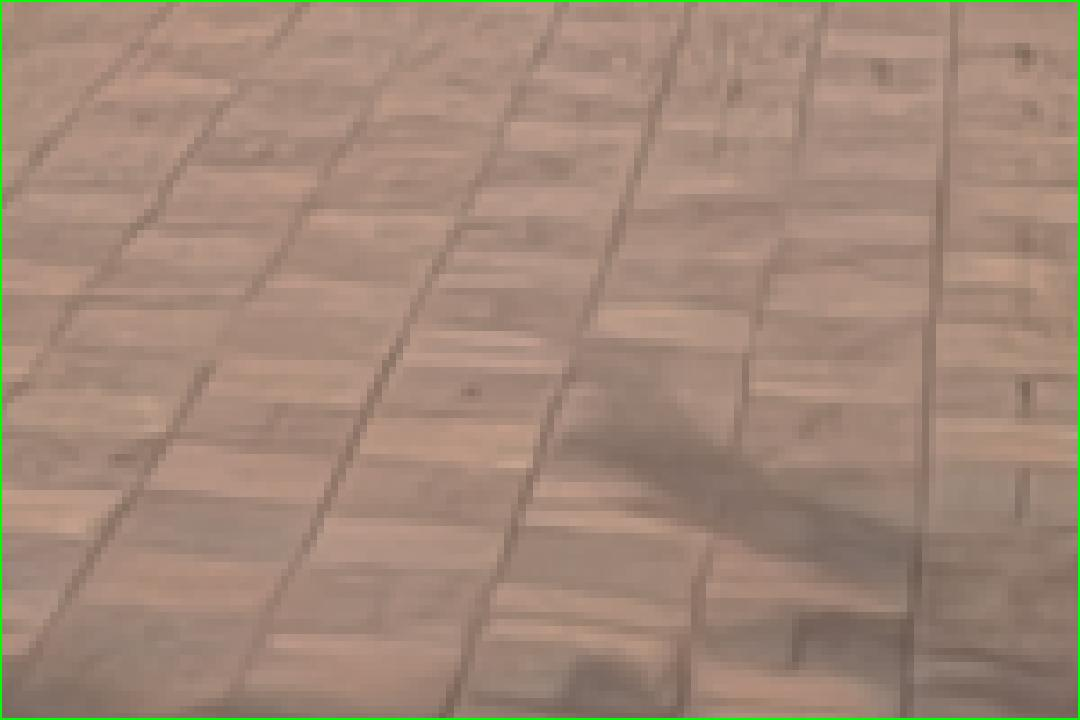}
    {\small (c) EDVR-VJDD~\cite{wang2019edvr}}
    \end{minipage} 
    \begin{minipage}[b]{0.24\textwidth}
    \centering
    \includegraphics[width=1\textwidth]{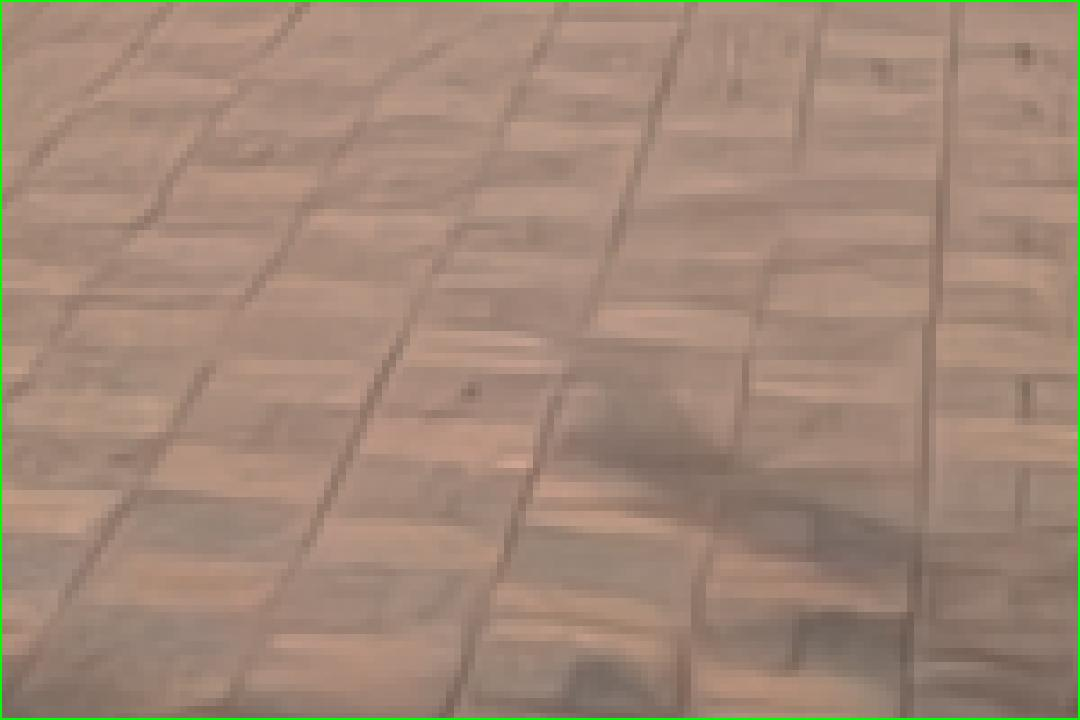}
    {\small (d) RviDeNet-VJDD~\cite{yue2020supervised}}
    \end{minipage} %\vspace{0.10cm}
\end{minipage}%\hspace{0.1cm}
\vspace{0.15cm}

\begin{minipage}[b]{0.95\textwidth}
\centering
%\hspace{4.42cm}
    \begin{minipage}[b]{0.24\textwidth}
    \centering
    \includegraphics[width=1\textwidth]{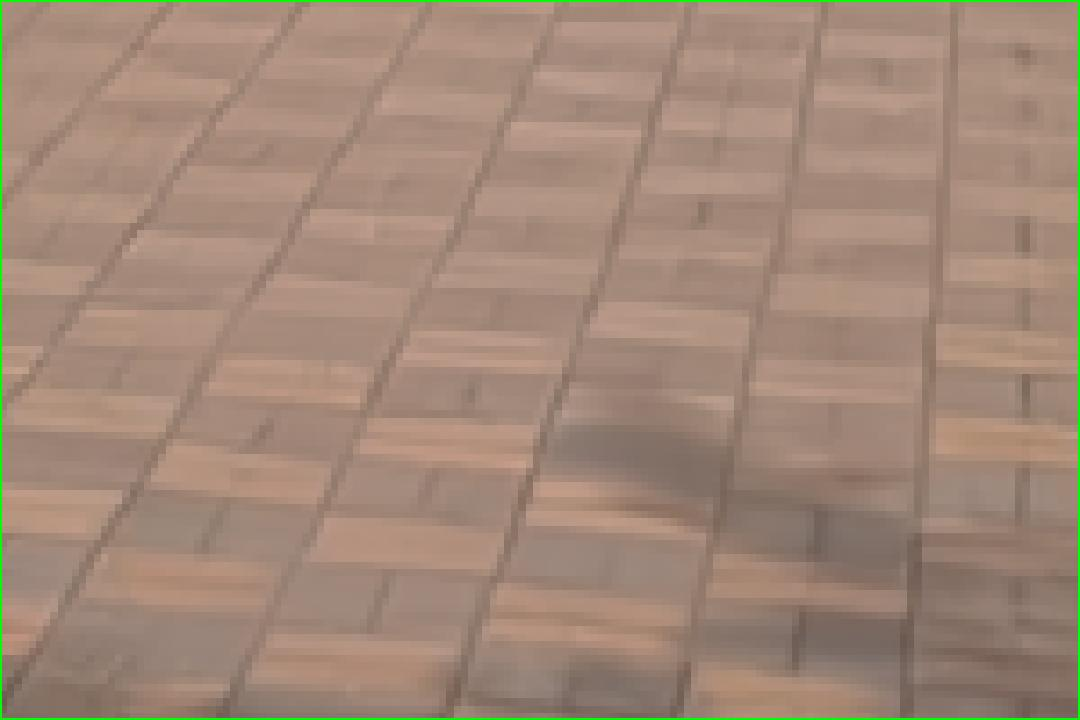}
    {\small (e) GCP-Net~\cite{guo2021joint}}
    \end{minipage} %\hspace{0.1cm}
    \begin{minipage}[b]{0.24\textwidth}
    \centering
    \includegraphics[width=1\textwidth]{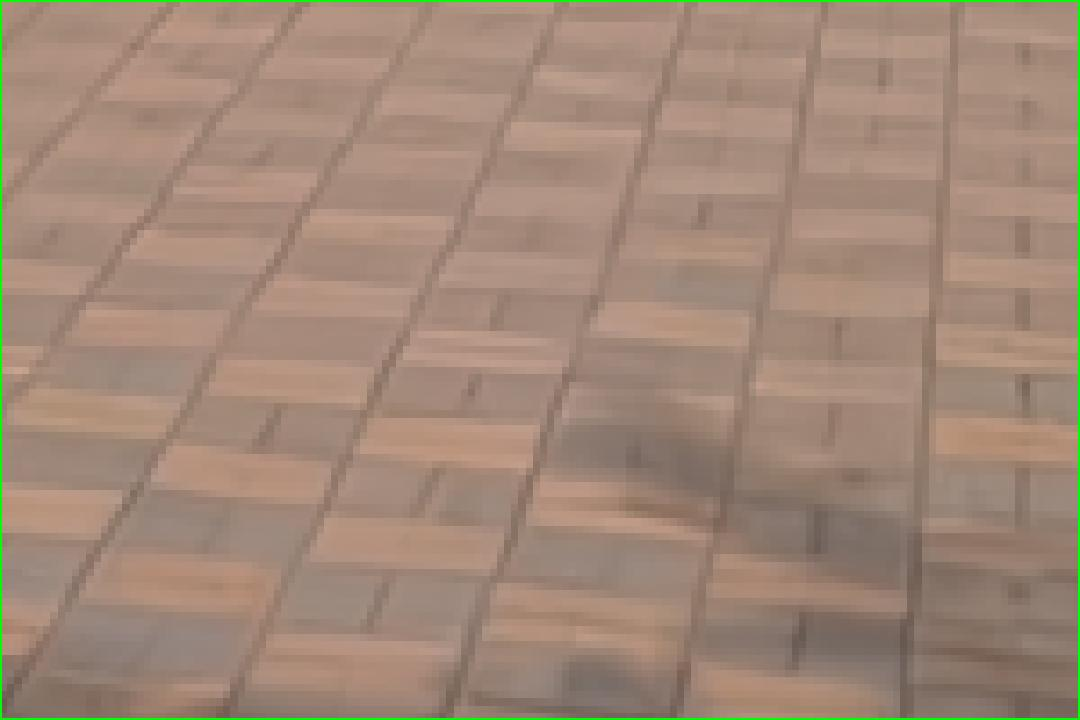}
    {\small (f) 2StageAlign~\cite{guo2022differentiable}}
    \end{minipage} %\hspace{0.1cm}
    \begin{minipage}[b]{0.24\textwidth}
    \centering
    \includegraphics[width=1\textwidth]{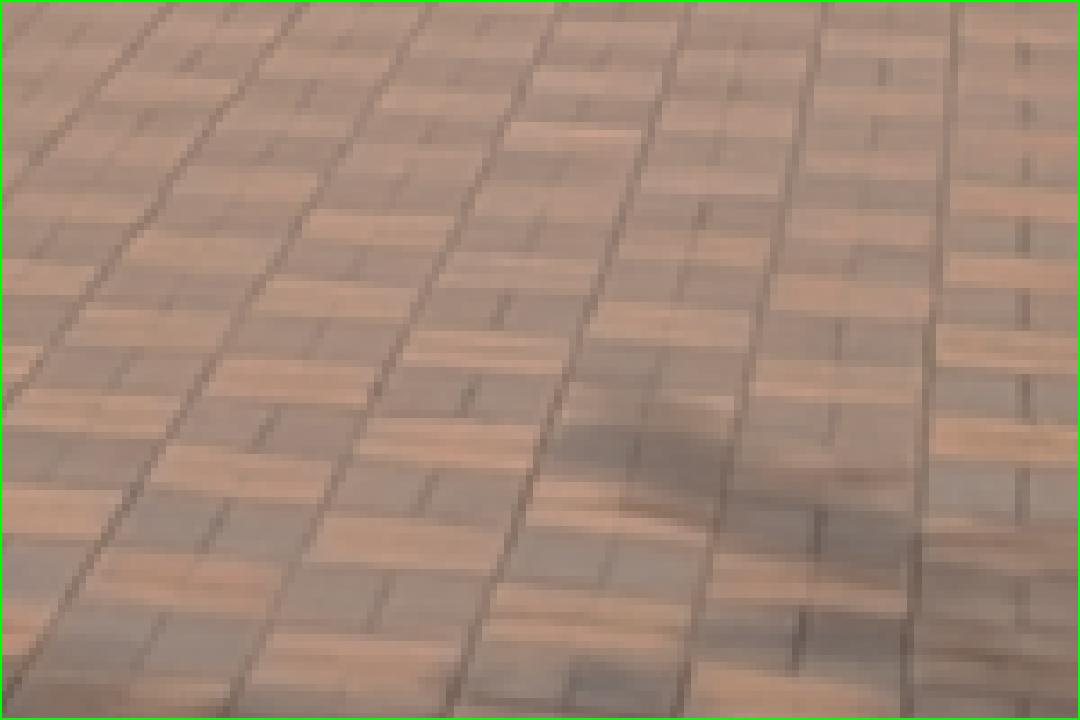}
    {\small (g) Ours}
    \end{minipage} %\hspace{0.1cm}
    \begin{minipage}[b]{0.24\textwidth}
    \centering
    \includegraphics[width=1\textwidth]{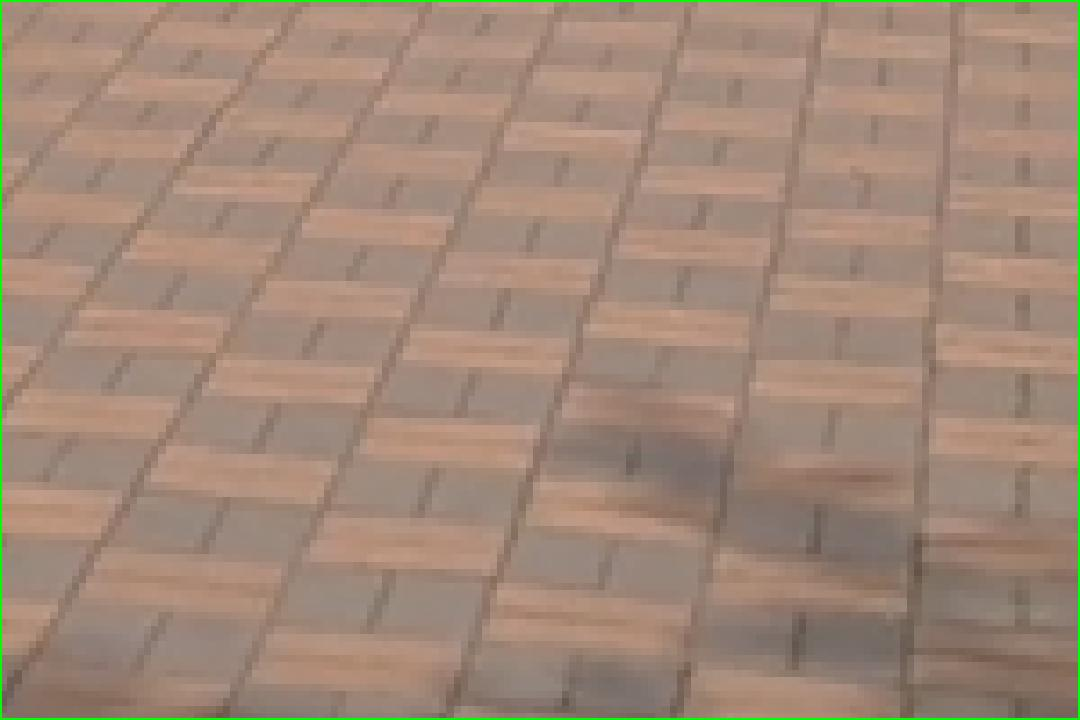}
    {\small (h) GT}
    \end{minipage} 
\end{minipage}%\hspace{0.1cm}
%\vspace{0.15cm}
\caption{VJDD results by different methods on \emph{Clip000} of the REDS4 dataset.}%\vspace{-0.4cm}
\label{fig:supp_Reds4_2}
\end{figure*}

% ----------- END FIGURE -----------

%%% -------- REDS4 results on high noise level: 03 --------
\begin{figure*}[!h]
\centering
% Patch 2
\begin{minipage}[b]{0.95\textwidth}
\centering
    \begin{minipage}[b]{0.24\textwidth}
    \centering
    \includegraphics[width=1\textwidth]{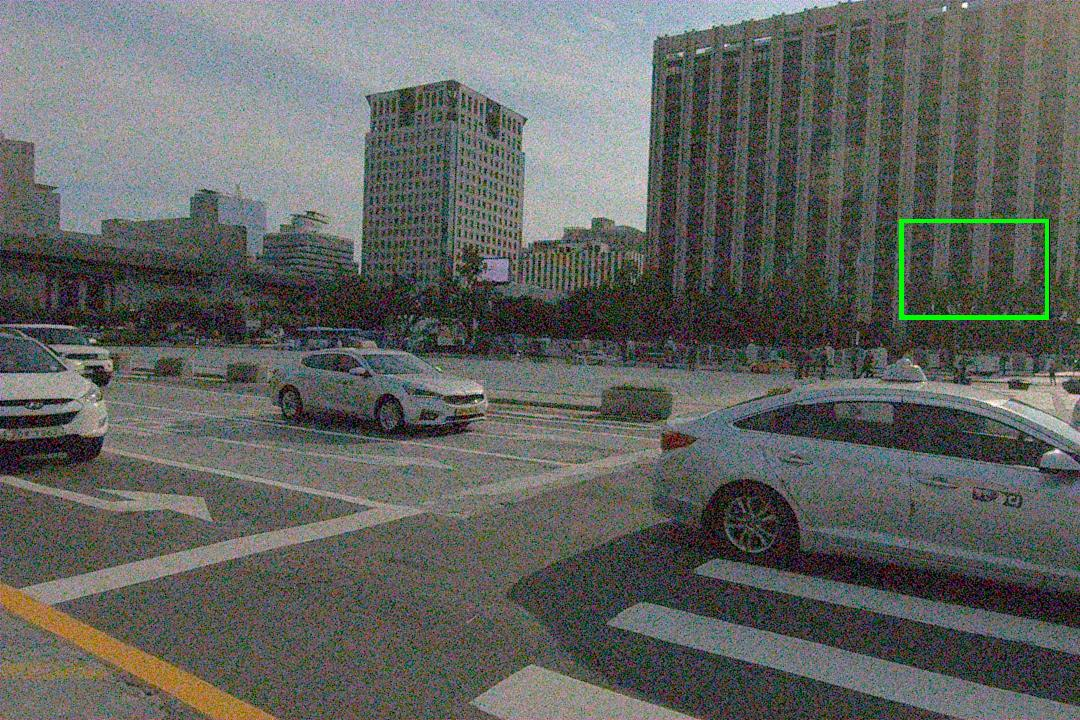}
    {\small (a) Noise image}
    \end{minipage} %\hspace{0.1cm}
    \begin{minipage}[b]{0.24\textwidth}
    \centering
    \includegraphics[width=1\textwidth]{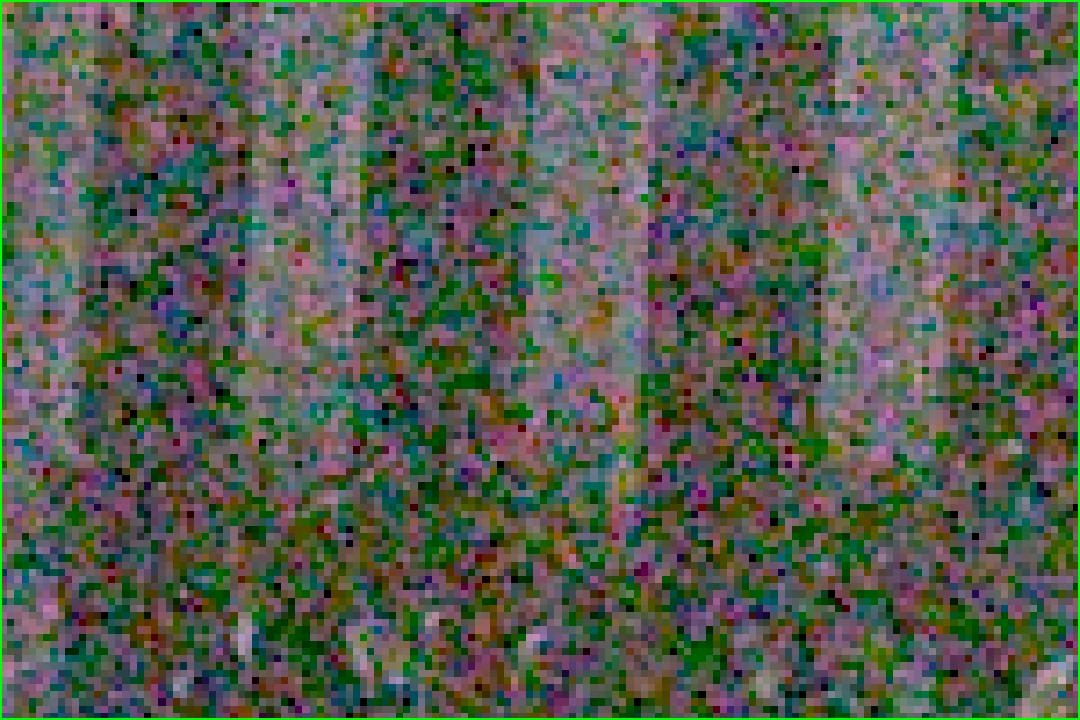}
    {\small (b) Noise patch}
    \end{minipage} %\hspace{0.1cm}
    \begin{minipage}[b]{0.24\textwidth}
    \centering
    \includegraphics[width=1\textwidth]{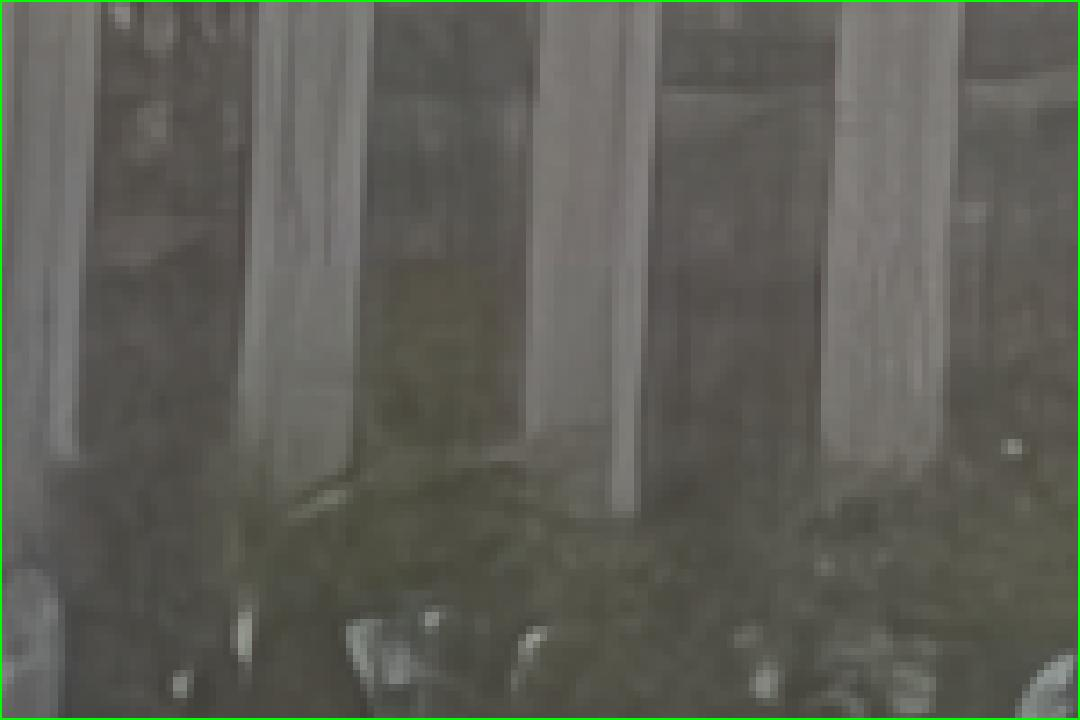}
    {\small (c) EDVR-VJDD~\cite{wang2019edvr}}
    \end{minipage} 
    \begin{minipage}[b]{0.24\textwidth}
    \centering
    \includegraphics[width=1\textwidth]{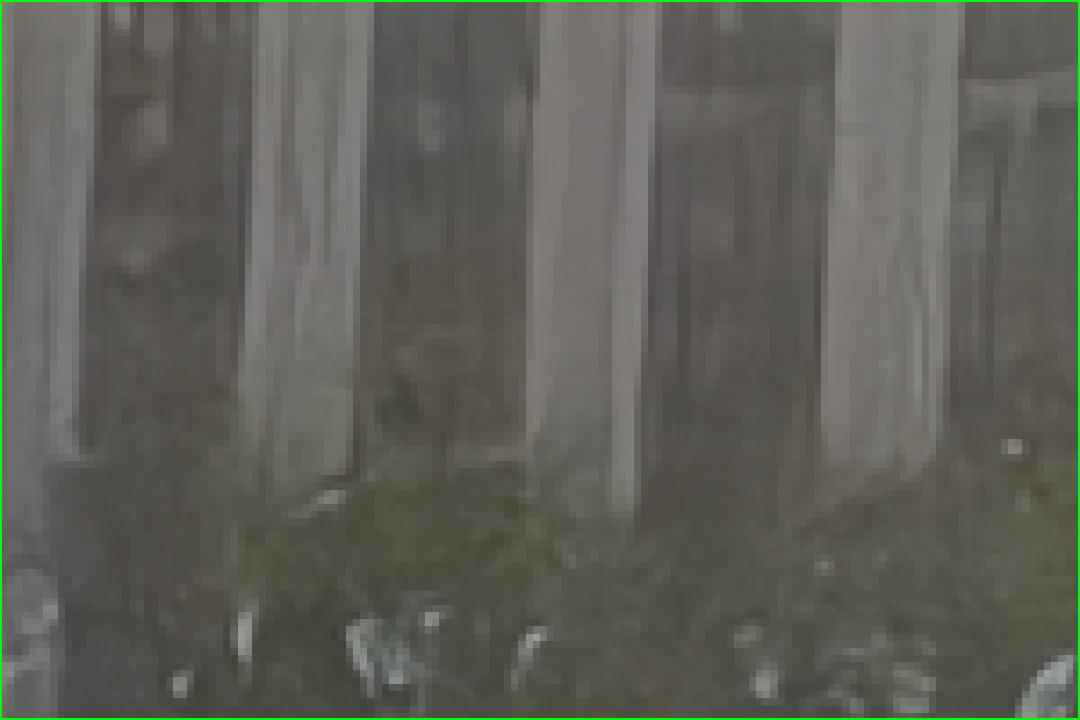}
    {\small (d) RviDeNet-VJDD~\cite{yue2020supervised}}
    \end{minipage} %\vspace{0.10cm}
\end{minipage}%\hspace{0.1cm}
\vspace{0.15cm}

\begin{minipage}[b]{0.95\textwidth}
\centering
%\hspace{4.42cm}
    \begin{minipage}[b]{0.24\textwidth}
    \centering
    \includegraphics[width=1\textwidth]{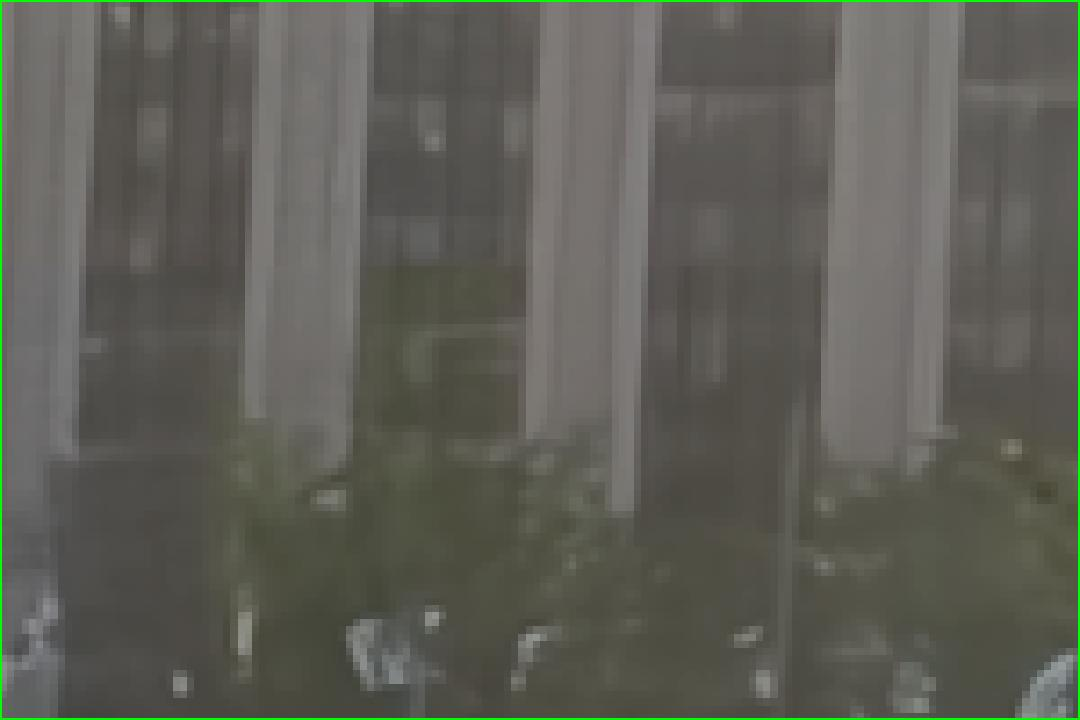}
    {\small (e) GCP-Net~\cite{guo2021joint}}
    \end{minipage} %\hspace{0.1cm}
    \begin{minipage}[b]{0.24\textwidth}
    \centering
    \includegraphics[width=1\textwidth]{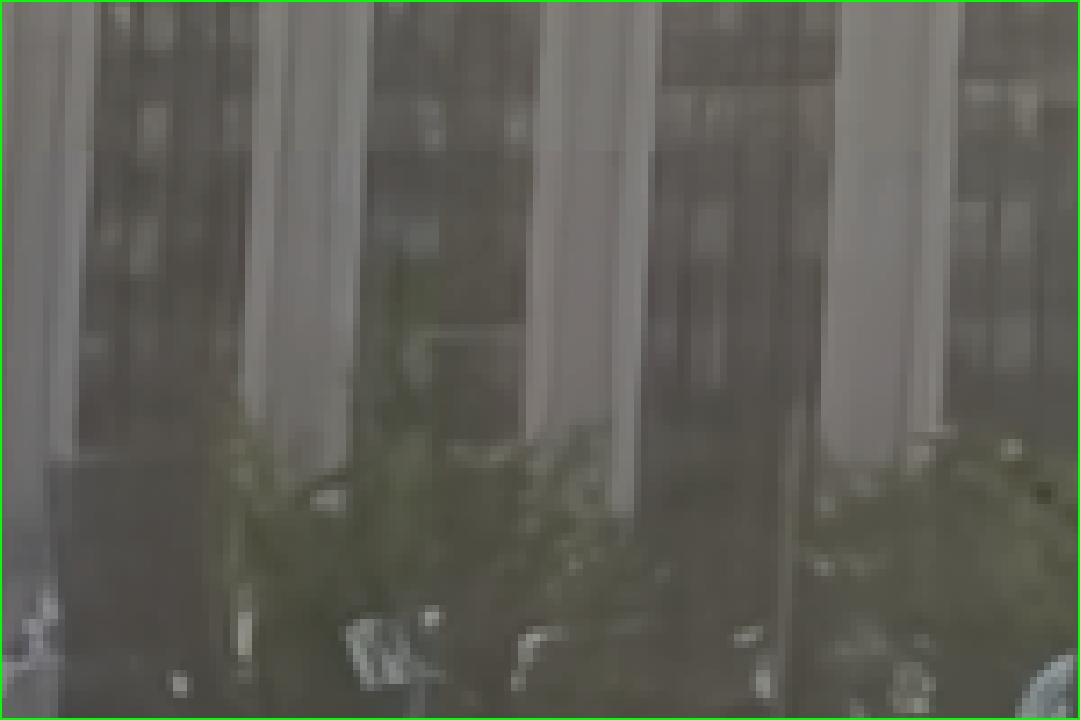}
    {\small (f) 2StageAlign~\cite{guo2022differentiable}}
    \end{minipage} %\hspace{0.1cm}
    \begin{minipage}[b]{0.24\textwidth}
    \centering
    \includegraphics[width=1\textwidth]{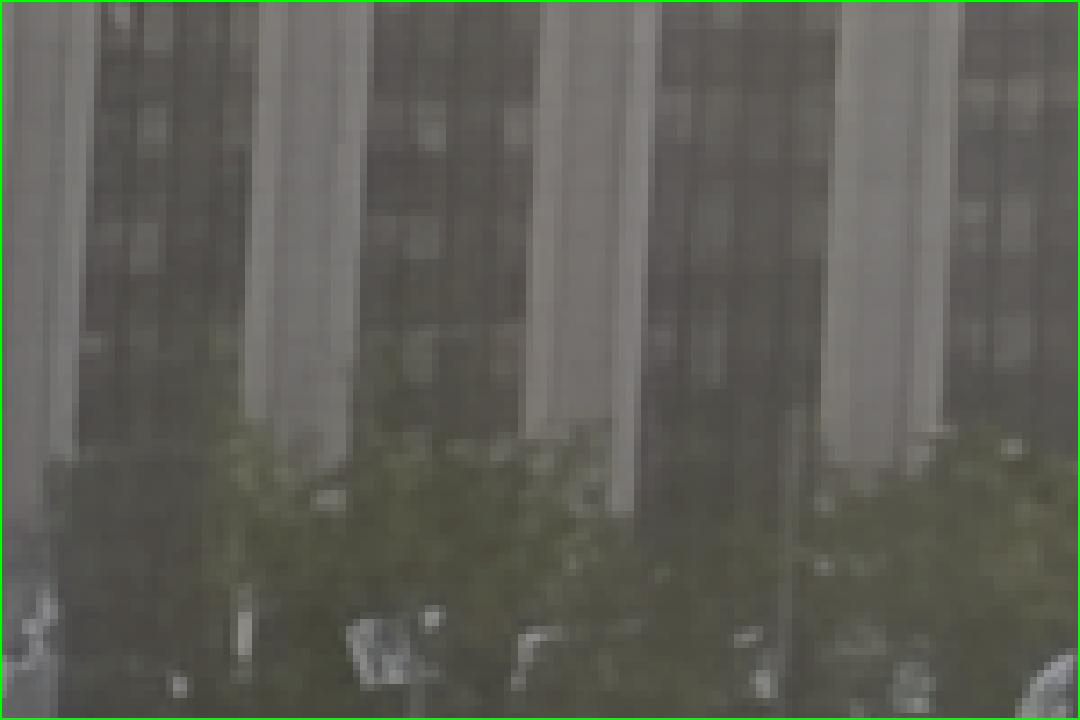}
    {\small (g) Ours}
    \end{minipage} %\hspace{0.1cm}
    \begin{minipage}[b]{0.24\textwidth}
    \centering
    \includegraphics[width=1\textwidth]{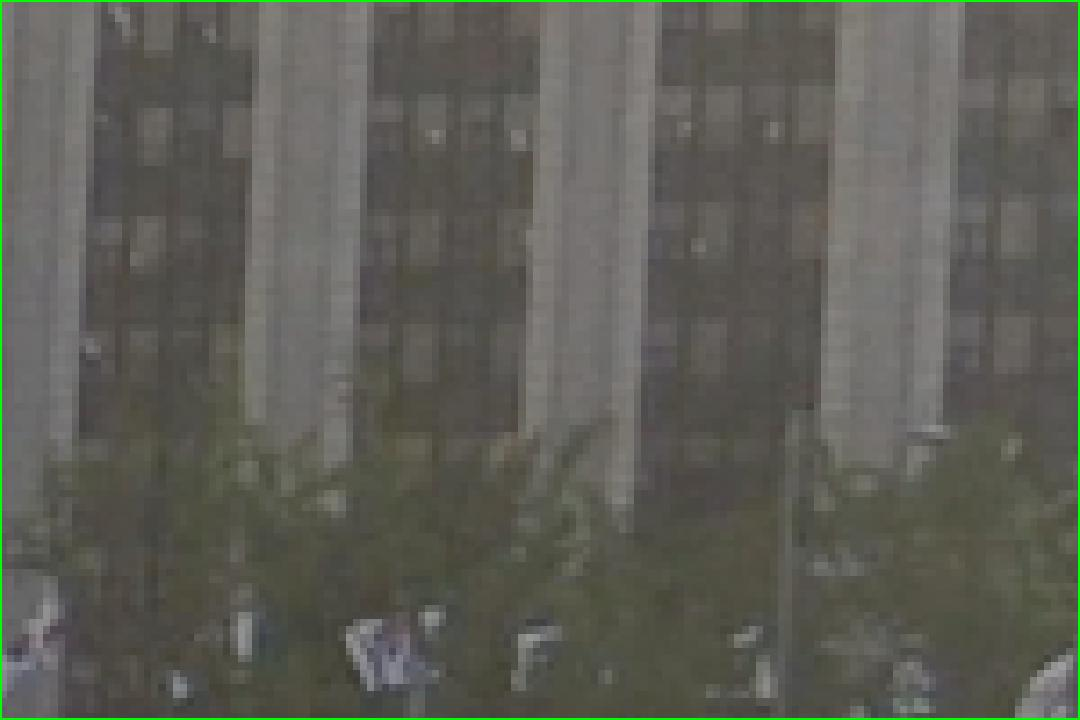}
    {\small (h) GT}
    \end{minipage} 
\end{minipage}%\hspace{0.1cm}
%\vspace{0.15cm}
\caption{VJDD results by different methods on \emph{Clip015} of the REDS4 dataset.}%\vspace{-0.4cm}
\label{fig:supp_Reds4_3}
\end{figure*}
% ----------- END FIGURE -----------

%%% -------- 4K results on high noise level: 02 --------
\begin{figure*}[!h]
\centering
% Patch 2
\begin{minipage}[b]{0.95\textwidth}
\centering
    \begin{minipage}[b]{0.24\textwidth}
    \centering
    \includegraphics[width=1\textwidth]{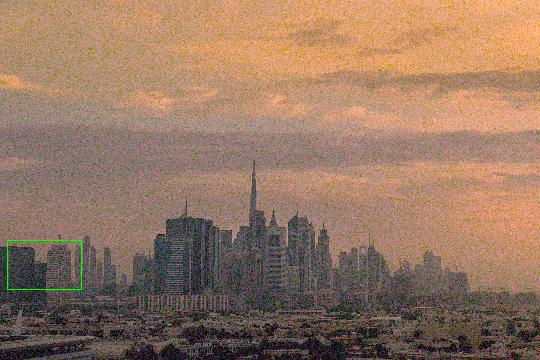}
    {\small (a) Noise image}
    \end{minipage} %\hspace{0.1cm}
    \begin{minipage}[b]{0.24\textwidth}
    \centering
    \includegraphics[width=1\textwidth]{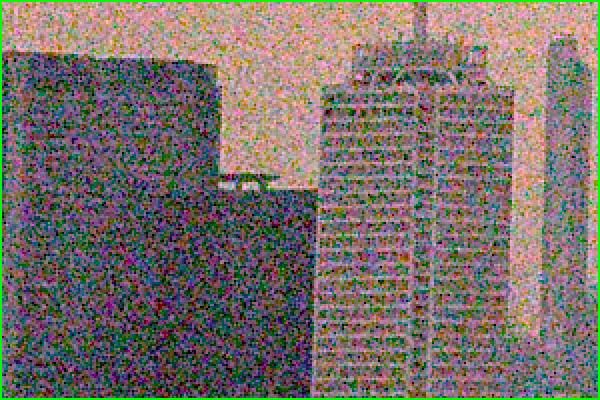}
    {\small (b) Noise patch}
    \end{minipage} %\hspace{0.1cm}
    \begin{minipage}[b]{0.24\textwidth}
    \centering
    \includegraphics[width=1\textwidth]{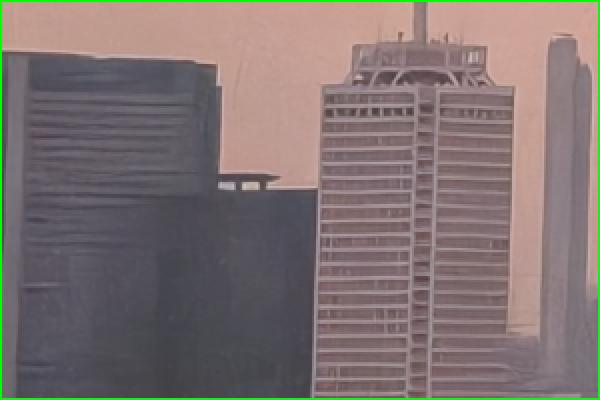}
    {\small (c) EDVR-VJDD~\cite{wang2019edvr}}
    \end{minipage} 
    \begin{minipage}[b]{0.24\textwidth}
    \centering
    \includegraphics[width=1\textwidth]{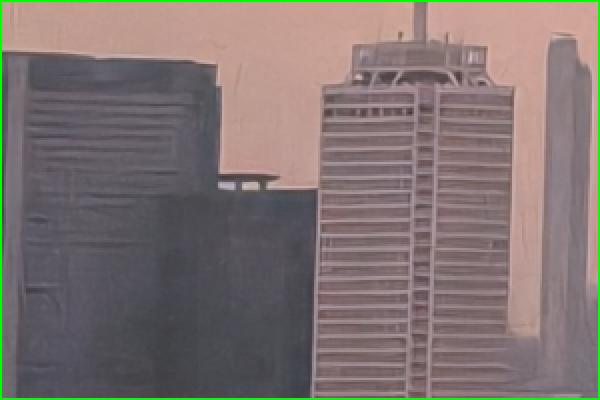}
    {\small (d) RviDeNet-VJDD~\cite{yue2020supervised}}
    \end{minipage} %\vspace{0.10cm}
\end{minipage}%\hspace{0.1cm}
\vspace{0.15cm}

\begin{minipage}[b]{0.95\textwidth}
\centering
%\hspace{4.42cm}
    \begin{minipage}[b]{0.24\textwidth}
    \centering
    \includegraphics[width=1\textwidth]{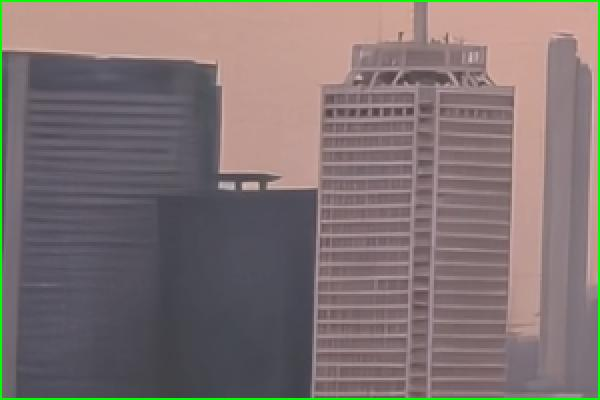}
    {\small (e) GCP-Net~\cite{guo2021joint}}
    \end{minipage} %\hspace{0.1cm}
    \begin{minipage}[b]{0.24\textwidth}
    \centering
    \includegraphics[width=1\textwidth]{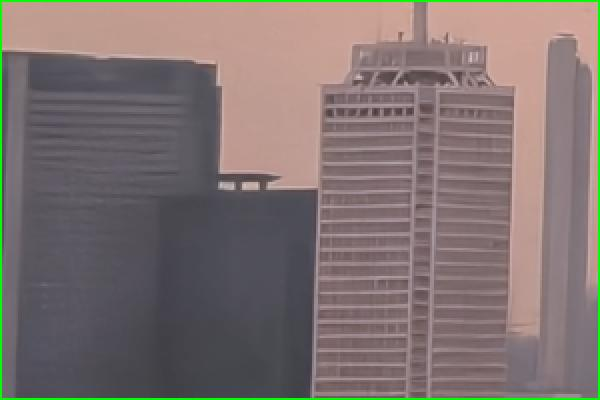}
    {\small (f) 2StageAlign~\cite{guo2022differentiable}}
    \end{minipage} %\hspace{0.1cm}
    \begin{minipage}[b]{0.24\textwidth}
    \centering
    \includegraphics[width=1\textwidth]{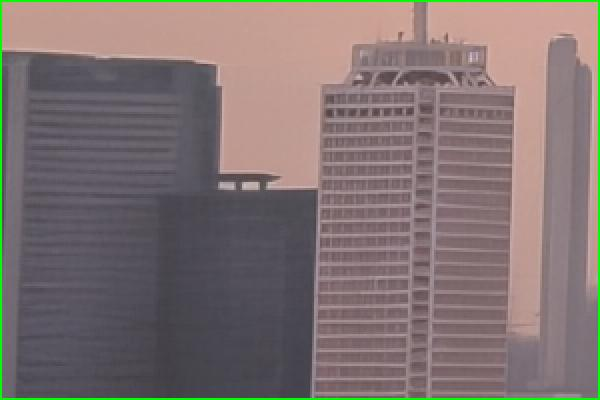}
    {\small (g) Ours}
    \end{minipage} %\hspace{0.1cm}
    \begin{minipage}[b]{0.24\textwidth}
    \centering
    \includegraphics[width=1\textwidth]{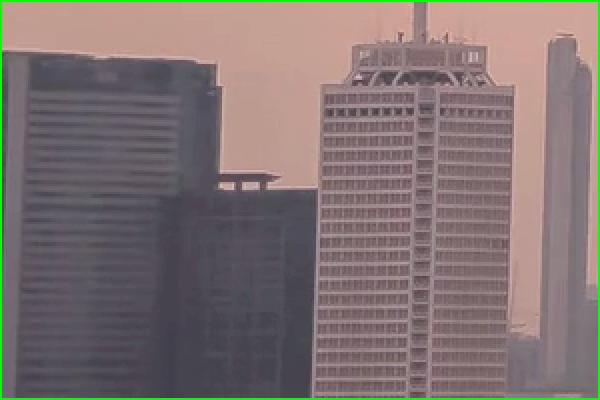}
    {\small (h) GT}
    \end{minipage} 
\end{minipage}%\hspace{0.1cm}
%\vspace{0.15cm}
\caption{VJDD results by different methods on 4KPix50 dataset.}%\vspace{-0.4cm}
\label{fig:supp_4kpix_1}
\end{figure*}
% ----------- END FIGURE -----------

%%% -------- 4K results on high noise level: 02 --------
\begin{figure*}[!h]
\centering
% Patch 2
\begin{minipage}[b]{0.95\textwidth}
\centering
    \begin{minipage}[b]{0.24\textwidth}
    \centering
    \includegraphics[width=1\textwidth]{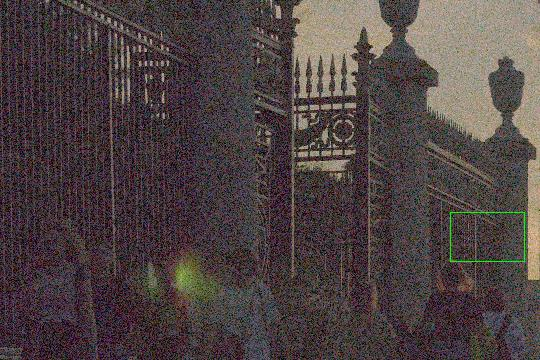}
    {\small (a) Noise image}
    \end{minipage} %\hspace{0.1cm}
    \begin{minipage}[b]{0.24\textwidth}
    \centering
    \includegraphics[width=1\textwidth]{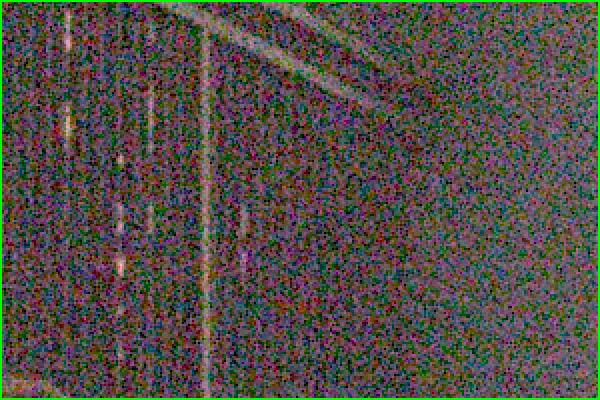}
    {\small (b) Noise patch}
    \end{minipage} %\hspace{0.1cm}
    \begin{minipage}[b]{0.24\textwidth}
    \centering
    \includegraphics[width=1\textwidth]{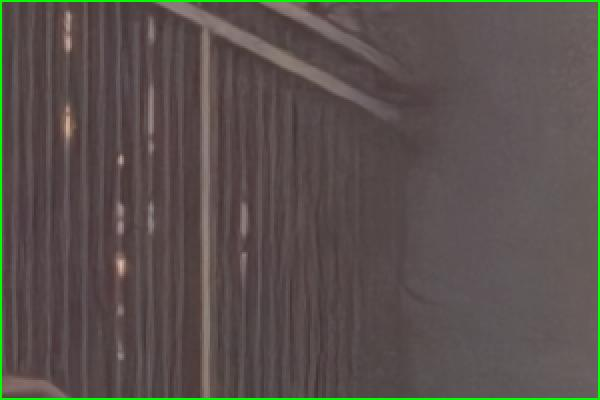}
    {\small (c) EDVR-VJDD~\cite{wang2019edvr}}
    \end{minipage} 
    \begin{minipage}[b]{0.24\textwidth}
    \centering
    \includegraphics[width=1\textwidth]{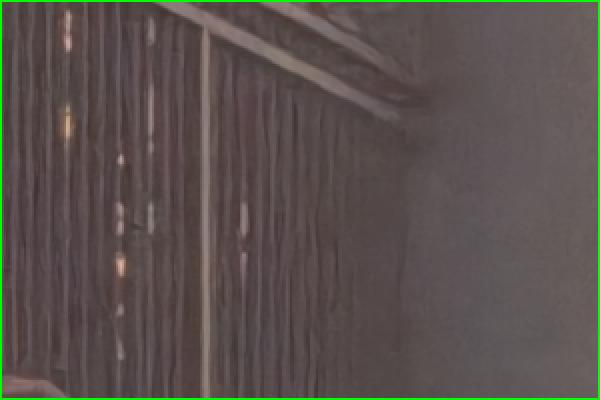}
    {\small (d) RviDeNet-VJDD~\cite{yue2020supervised}}
    \end{minipage} %\vspace{0.10cm}
\end{minipage}%\hspace{0.1cm}
\vspace{0.15cm}

\begin{minipage}[b]{0.95\textwidth}
\centering
%\hspace{4.42cm}
    \begin{minipage}[b]{0.24\textwidth}
    \centering
    \includegraphics[width=1\textwidth]{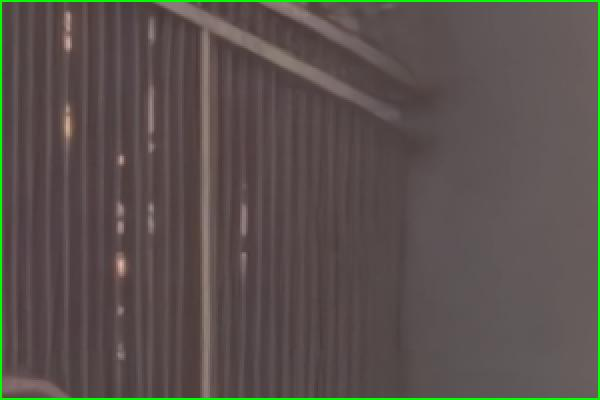}
    {\small (e) GCP-Net~\cite{guo2021joint}}
    \end{minipage} %\hspace{0.1cm}
    \begin{minipage}[b]{0.24\textwidth}
    \centering
    \includegraphics[width=1\textwidth]{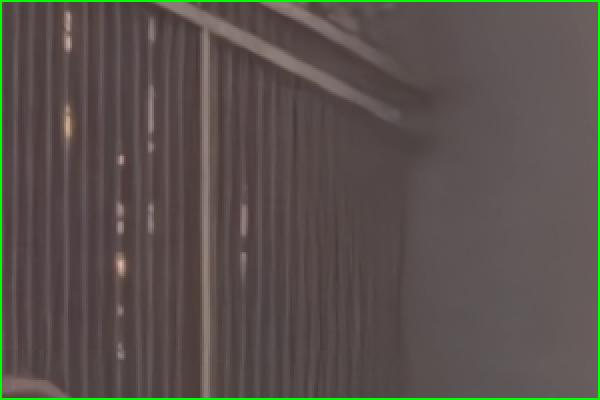}
    {\small (f) 2StageAlign~\cite{guo2022differentiable}}
    \end{minipage} %\hspace{0.1cm}
    \begin{minipage}[b]{0.24\textwidth}
    \centering
    \includegraphics[width=1\textwidth]{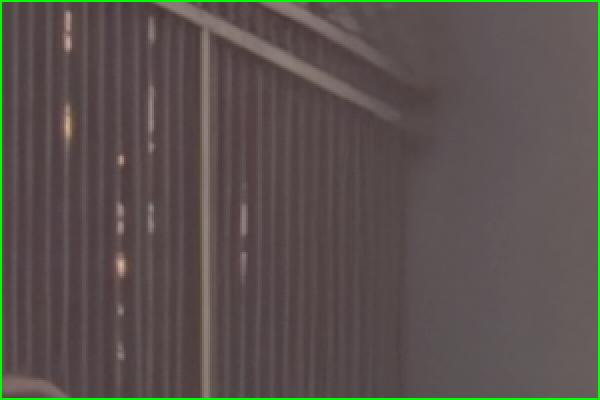}
    {\small (g) Ours}
    \end{minipage} %\hspace{0.1cm}
    \begin{minipage}[b]{0.24\textwidth}
    \centering
    \includegraphics[width=1\textwidth]{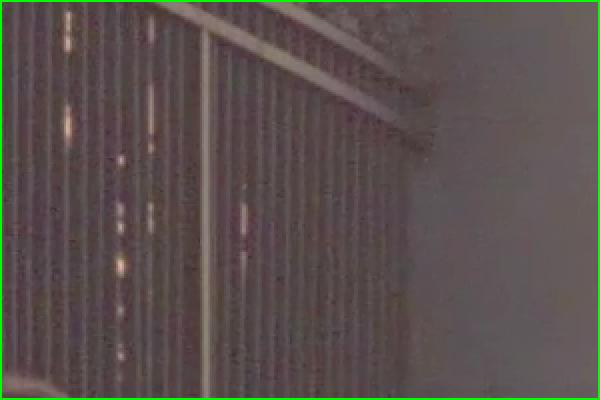}
    {\small (h) GT}
    \end{minipage} 
\end{minipage}%\hspace{0.1cm}
%\vspace{0.15cm}
\caption{VJDD results by different methods on 4KPix50 dataset.}%\vspace{-0.4cm}
\label{fig:supp_4kpix_2}
\end{figure*}
% ----------- END FIGURE -----------
